# Supplementary material for: Predicting Change, Not States: An Alternate Framework for Neural PDE Surrogates
Source: arXiv:2412.13074 source file (2025-04-16)
Supplement: Supplementary file 1 [file supplementaryinfo.tex]

Appendix
